# Supplementary material for: SeMask: Semantically Masked Transformers for Semantic Segmentation
Source: arXiv:2112.12782 source file (2022-04-13)
Supplement: Supplementary file 1 [file limitations.tex]

\section{Limitations}

The inclusion of SeMask Blocks in the hierarchical vision transformer backbones helps us to incorporate a local inductive bias into the network. However, CNNs already have a strong local inductive bias due to the translation-invariant convolution operation, while the transformers have a lack of the same \cite{vit-cnn}. Our experiments with CNNs suggest that the proposed module harms the performance when added to CNN networks. This could be due to the difference in the layer-wise learning nature of transformers and CNN networks, ViT \cite{vit} has both local and global heads even in the lowest layers, unlike CNNs which attend only locally in the lower layers \cite{vit-cnn}. We plan to conduct a more comprehensive study with the CNNs in the future.
